# Supplementary material for: Higher Josephson harmonics in a tunable double-junction transmon qubit
Source: arXiv:2512.08470 source file (2026-07-21)
Supplement: Supplementary file 1 [file preamble_SI.tex]

% ****** Start of file apssamp.tex ******
%
%   This file is part of the APS files in the REVTeX 4.2 distribution.
%   Version 4.2a of REVTeX, December 2014
%
%   Copyright (c) 2014 The American Physical Society.
%
%   See the REVTeX 4 README file for restrictions and more information.
%
% TeX'ing this file requires that you have AMS-LaTeX 2.0 installed
% as well as the rest of the prerequisites for REVTeX 4.2
%
% See the REVTeX 4 README file
% It also requires running BibTeX. The commands are as follows:
%
%  1)  latex apssamp.tex
%  2)  bibtex apssamp
%  3)  latex apssamp.tex
%  4)  latex apssamp.tex
%
\documentclass[aps,prl,onecolumn,superscriptaddress]{revtex4-2}

%reprint,
%superscriptaddress,
%groupedaddress,
%unsortedaddress,
%runinaddress,
%frontmatterverbose, 
%preprint,
%preprintnumbers,
%nofootinbib,
%nobibnotes,
%bibnotes,
%amsmath,
%amssymb,
%aps,
%pra,
%prb,
%rmp,
%prstab,
%prstper,
%floatfix,

\usepackage{siunitx}
\usepackage{graphicx}% Include figure files
\usepackage{dcolumn}% Align table columns on decimal point
\usepackage{bm}% bold math
\usepackage{braket}
\usepackage{amsmath}
\usepackage{amssymb}
%\usepackage{hyperref}% add hypertext capabilities
%\usepackage[mathlines]{lineno}% Enable numbering of text and display math
%\linenumbers\relax % Commence numbering lines
%\usepackage[showframe,%Uncomment any one of the following lines to test 
%%scale=0.7, marginratio={1:1, 2:3}, ignoreall,% default settings
%%text={7in,10in},centering,
%%margin=1.5in,
%%total={6.5in,8.75in}, top=1.2in, left=0.9in, includefoot,
%%height=10in,a5paper,hmargin={3cm,0.8in},
%]{geometry}
\usepackage{comment}
\usepackage{hyperref}
\usepackage{cleveref}
\usepackage{subfiles}
\usepackage{tikz}
\newcommand{\mk}[1]{{\color{red}#1}} %Morten Kjaergaard
\newcommand{\jj}{%
  \tikz[baseline=-0.6ex, x=1em, y=1em, yshift=-0.7pt]{%
    \def\s{0.18}   % half-side of each square
    \def\sep{0.6} % center-to-center distance between the two JJs
    \def\lead{0.35}% lead length at both ends

    % left lead to first square
    \draw (-\lead,0) -- (-\s,0);

    % first JJ at x = 0
    \draw (-\s,-\s) rectangle (\s,\s);
    \draw (-\s,-\s) -- (\s,\s);
    \draw (-\s,\s) -- (\s,-\s);

    % wire between first and second JJ:
    % first square ends at x = +\s, second square (center \sep) begins at x = \sep - \s
    \draw (\s,0) -- (\sep-\s,0);

    % second JJ, centered at x = \sep
    \begin{scope}[xshift=\sep em]
      \draw (-\s,-\s) rectangle (\s,\s);
      \draw (-\s,-\s) -- (\s,\s);
      \draw (-\s,\s) -- (\s,-\s);
    \end{scope}

    % right lead from second square
    \draw (\sep+\s,0) -- (\sep+\lead,0);
  }%
}
